# Supplementary material for: First simultaneous measurement of differential muon-neutrino charged-current cross sections on argon for final states with and without protons using MicroBooNE data
Source: arXiv:2402.19281 ancillary file (2024-07-27)
Supplement: Supplementary file 1 [file SupplementalMaterial.pdf]

# Supplemental Material for “First simultaneous measurement of differential muon-neutrino charged-current cross sections on argon for final states with and without protons using MicroBooNE data”

This Letter shares the same event reconstruction, event selection, model validation, fake data studies, systematics and unfolding procedure as [1]. Additional details and studies can be found there and in its accompanying Supplemental Material. The data release is identical in this Letter and [1] and includes measurements from both manuscripts. A single covariance matrix is included in this data release. It contains inter-variable correlations as is obtained with the blockwise formulation of the unfolding described in [2] and in the main text of [1]. More details on the data release are in Sec. IV.

## I. 2D SMEARING AND EFFICIENCIES

The section presents the smearing matrices for the 2D  $\{\cos\theta_\mu^{rec}, E_\mu\}$  distribution. The efficiency of the  $\nu_\mu$ CC selection as a function of the same variables is also shown. The binning used for these plots is the same as used for  $S$  in the cross section extraction and is identical between reconstructed and true bins. All bins are equal width and do not represent the physical width of the energy and angle bins. The bins are in angular slices that go from backwards on the left to forwards on the right with increasing energy bins within each slice. More information on the binning can be found in Sec. IV.

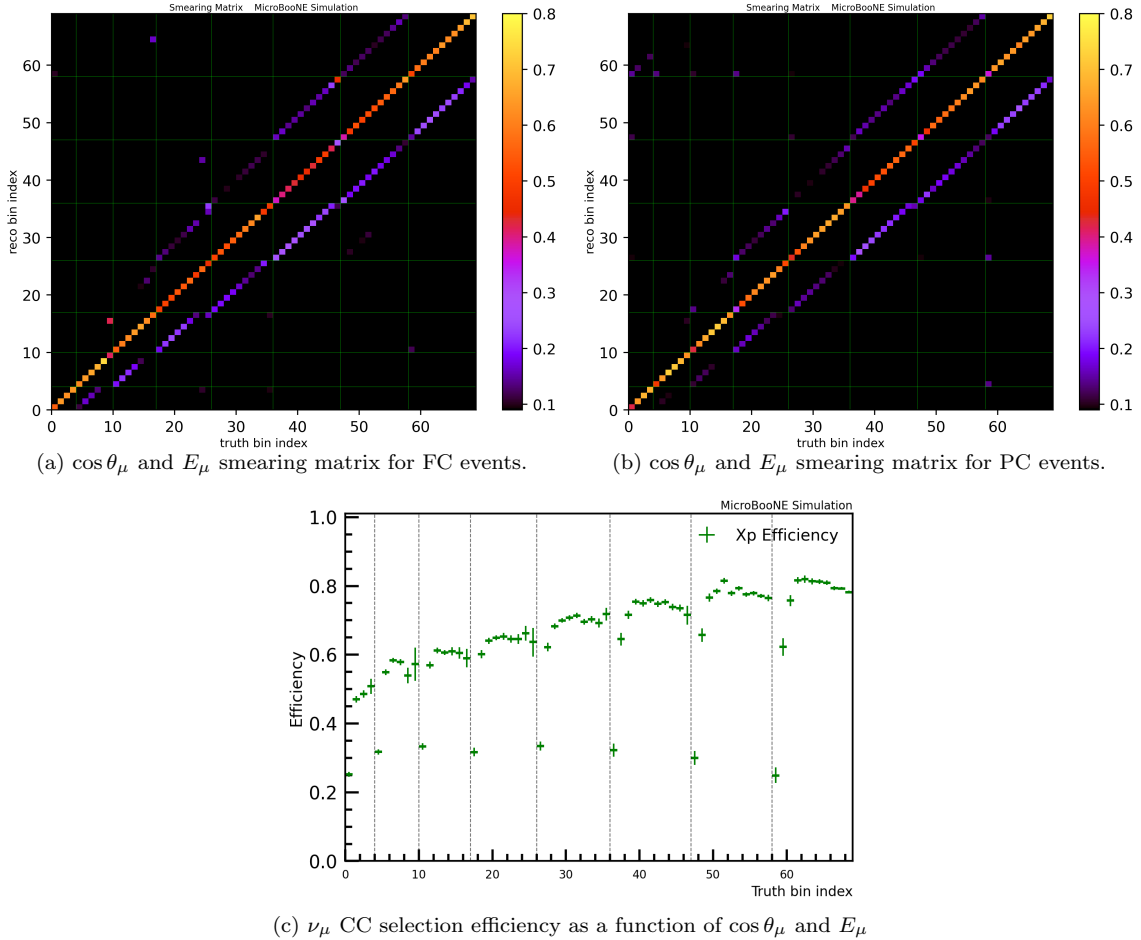

FIG. 1: Smearing matrix for the double differential measurement of  $\cos\theta_\mu$  and  $E_\mu$  for FC events (a) and PC events (b). All columns have been normalized to one. The green lines indicate the different angular slices. (c) Vectors efficiency of the  $\nu_\mu$ CC selection for each true  $\cos\theta_\mu$  and  $E_\mu$  bin in the double differential measurement. The dotted lines indicate the different angular slices. In all plots, the true and reconstructed bins are the same as those on  $S$  in the cross section extraction but are all equal width and do not represent the physical width of the energy and angle bins.

## II. FAKE DATA STUDIES

Fake data studies (FDS) were conducted to test the robustness of the model validation, derivation of the additional reweighting uncertainty and cross section extraction. For the FDS presented here, a NuWro MC sample was propagated through the MicroBooNE simulation and reconstruction chain in the same way as the nominal  $\mu$ BooNE tune MC, after which it is treated identically to real data. The purpose of this FDS is to serve as a case study of how the model validation is able to detect relevant mismodeling thereby allowing it to be mitigated via the addition of a (fake-)data-driven reweighting uncertainty obtained as described in Sec. VII of [1]. With this overall procedure, the cross section results presented in this study were not biased beyond their uncertainties. Note that the additional uncertainty derived for this FDS is not applied to real data, it is specific to the context of this FDS.

Because the fake data and MC prediction use the same detector and flux simulations, uncertainties due to beam exposure, number of targets, detector, fluxes, and reinteractions are fully correlated and thus somewhat superficial. For these tests, only the uncorrelated uncertainties (cross section, statistical, and MC statistical) are used for the model validation, the cross section extraction, and the subsequent  $\chi^2$  calculations between the fake data results and generator predictions. The removal of these fully correlated uncertainties provides a more direct test of the cross section model and its relation to the model validation procedure and cross section extraction. Since the conditional constraint tests used for validation are agnostic to the source of uncertainty, it is perhaps more useful to probe the ability of the validation to detect relevant mismodeling with a treatment of the uncertainty more akin to that of real data. Such studies, which are designed to more directly probe the ability of the model validation to detect relevant mismodeling, are presented in the Supplemental Material of [1].

The same model validation used for real data was applied to the fake data in this study. These tests expose significant disagreement between the NuWro fake data and MC prediction in the hadronic final states. This can be seen in Fig. 2(a) which shows that, analogously to real data, the  $\mu$ BooNE tune MC is unable to describe the NuWro fake data within its uncertainties. Thus, the model should be expanded before it is used to extract the desired cross sections. Using the procedure described in Sec. VII of [1], an additional reweighting uncertainty is obtained from a reweighting function derived by unfolding the fake data with a constrained background and signal prediction and only the statistical uncertainties. This reweighting function can be seen in Fig. 2(b) alongside the one obtained from real data. The additional covariance matrix is then constructed in the same way as  $V_{\text{xs}}$  by treating the reweighted prediction as a  $1\sigma$  deviation from the original MC prediction. With this additional uncertainty applied to the MC prediction, the model shows an improved ability to describe the fake data. This can be seen in Fig. 2(c).

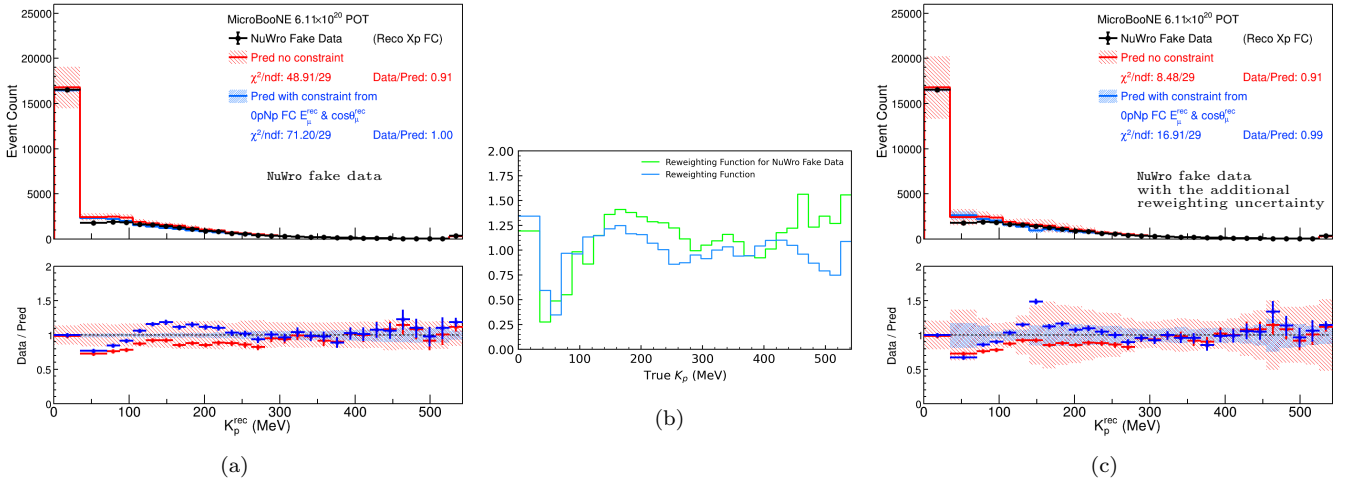

FIG. 2: (a) Fake data model validation for  $K_p^{\text{rec}}$ . Only the cross section and statistical uncertainties are included in the constraint from the muon kinematics and the calculation of the  $\chi^2$  values. This distribution does not pass model validation and motivates deriving a reweighting function to apply additional uncertainty to the fake data. This reweighting function can be seen in (b) next to the one for real data. (c) shows the same  $K_p^{\text{rec}}$  distribution and constraint as (a), but with the addition of reweighting systematic applied. The improved  $\chi^2$  shows that the reweighting is sufficient for  $K_p^{\text{rec}}$ .

The results of the  $K_p$  and 0pNp  $E_\mu$  and  $\cos \theta_\mu$  double-differential fake data cross section extractions are presented in Figs. 3 and 4. These plots contain the extracted fake data differential cross section as well as NuWro 19.02.2 (NuWro),  $\mu$ BooNE tune, GiBUU 2023 (GiBUU), GENIE v3.0.6 G18\_10a\_02\_11a (GENIE), and NEUT 5.4.0.1 (NEUT) predictions. Each generator prediction has been smeared with the  $A_C$  matrix obtained from unfolding the fake data. The NuWro prediction corresponds to the same generator configuration as used to produce the fake data but was generated independently and at higher stats than the fake data, which, at  $6.11 \times 10^{20}$  POT, is comparable in size to the real data set. Thus closure of these fake data studies is achieved when the extracted result shows good agreement with this prediction. This is indeed the case in Figs. 3 and 4, with the extracted fake data cross section agreeing better with the NuWro prediction (red dotted line) than with any other generator. The 0p, Np and 0pNp  $\chi^2/ndf$  values are also around or below unity and the NuWro prediction falls within  $1\sigma$  of the extracted results on almost all bins. The success of these fake data studies serve as an example of how the model validation and subsequent model expansion can be used to mitigate the potential for biased cross section results. Together, these fake data studies and the ones presented in the Supplemental Material of [1] serve as a thorough test of the model validation, model expansion, and unfolding, giving us confidence that our overall methodology is robust.

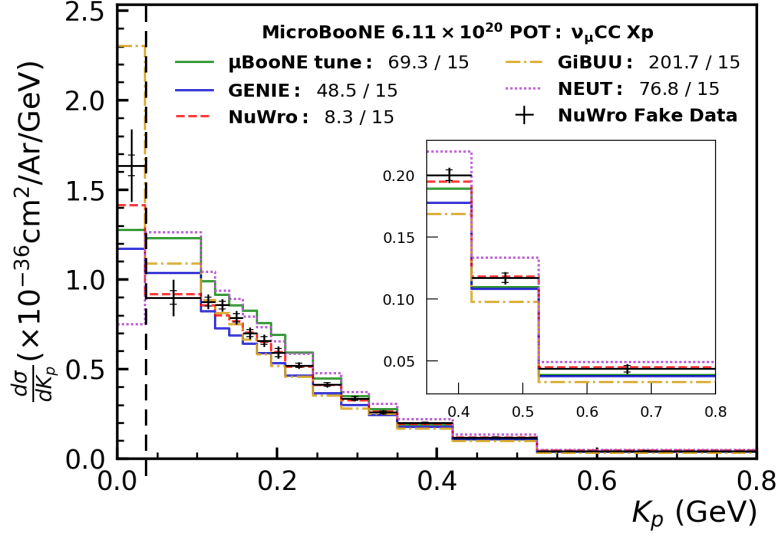

FIG. 3: Unfolded NuWro fake data  $K_p$  differential cross section result. The dashed line indicates the 35 MeV proton tracking threshold, below which is a single bin that includes events with no protons and events where the leading proton is below the threshold. The inner error bars on the data points represent the data statistical uncertainty, and the outer error bars represent the total uncorrelated uncertainty, which includes only the statistical, cross section and reweighting systematics, given by the square root of the diagonal elements of the extracted covariance matrix. Different generator predictions are indicated by the colored lines with corresponding  $\chi^2$  values displayed in the legend. The inset show a magnified view of the last three bins.

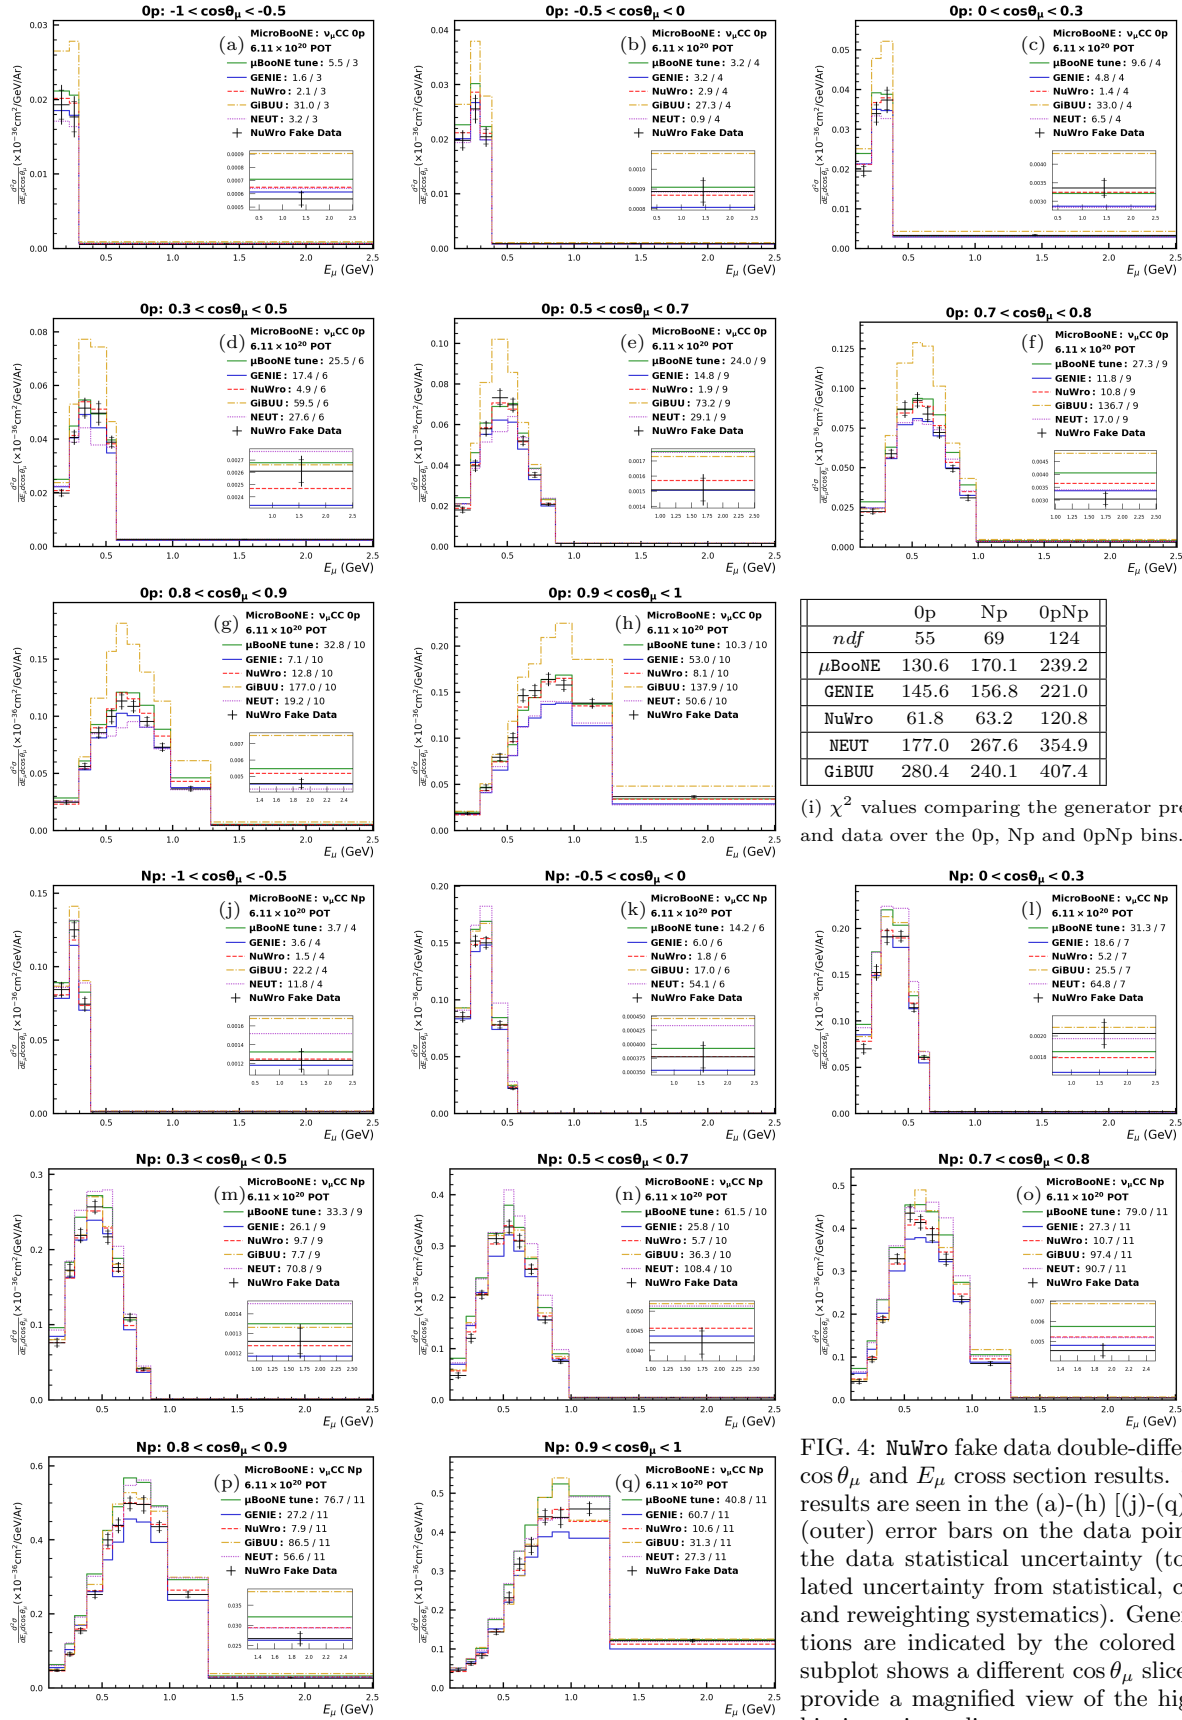

FIG. 4: NuWro fake data double-differential 0pNp  $\cos \theta_\mu$  and  $E_\mu$  cross section results. The 0p (Np) results are seen in the (a)-(h) [(j)-(q)]. The inner (outer) error bars on the data points represent the data statistical uncertainty (total uncorrelated uncertainty from statistical, cross section, and reweighting systematics). Generator predictions are indicated by the colored lines. Each subplot shows a different  $\cos \theta_\mu$  slice. The insets provide a magnified view of the highest energy bin in a given slice.

### III. SINGLE-DIFFERENTIAL MEASUREMENTS

Analogous to the Xp double-differential measurement seen in Fig. 1(a) of the main text, the single-differential  $\cos \theta_\mu$  and  $E_\mu$  cross section measurements are presented in this section. The  $E_\mu$  result can be seen in Fig. 5 and the  $\cos \theta_\mu$  result can be seen in Fig. 6. The single-differential 0pNp measurements analogous to the double-differential ones seen in Figs. 1(b) and 1(c) of the main text can be found in [1].

Similar to the double-differential case, the single-differential Xp cross section results look fairly similar to the Np ones due to the larger Np cross section. Nevertheless, the single-differential Xp results display some differences compared to the 0pNp results in term of agreement with generators. These differences are consistent with what is observed for the double-differential measurements. In particular, as seen in Fig. 6, NEUT describes the data best for Xp  $\cos \theta_\mu$ , but the worst for 0pNp  $\cos \theta_\mu$ . Conversely, GiBUU describes Xp  $\cos \theta_\mu$  noticeably worse than 0pNp. NEUT also does significantly better for Xp  $E_\mu$  than for 0pNp  $E_\mu$ , though GiBUU and the  $\mu$ BooNE tune offer similar levels of agreement, which can be seen in Fig. 5. The underprediction of all generators at the peak of the  $E_\mu$  distribution appears more prominent for the Xp measurement than the Np one, which is not surprising due to the consistent observation of the feature in the Np channel and consistent observation of a data excess for all but GiBUU in the 0p channel.

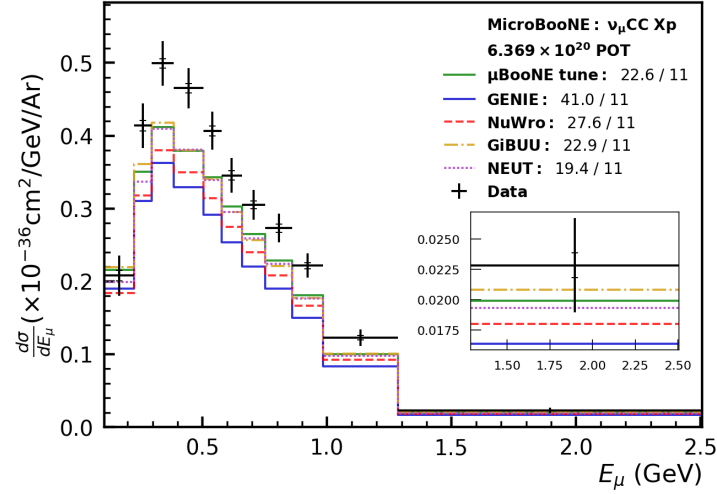

FIG. 5: Unfolded Xp  $E_\mu$  differential cross section result. The inner error bars on the data points represent the data statistical uncertainty, and the outer error bars represent the total uncorrelated uncertainty given by the square root of the diagonal elements of the extracted covariance matrix. Different generator predictions are indicated by the colored lines with corresponding  $\chi^2$  values displayed in the legend. The inset provides a magnified view of the most energetic bin.

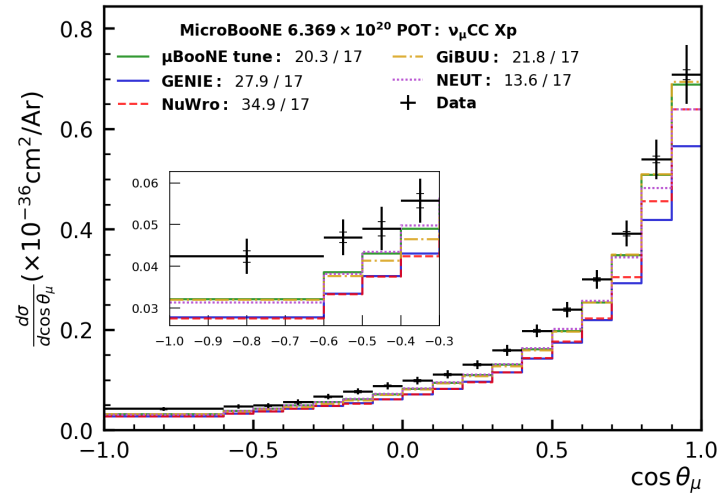

FIG. 6: Unfolded Xp  $\cos \theta_\mu$  differential cross section result. The inner error bars on the data points represent the data statistical uncertainty, and the outer error bars represent the total uncorrelated uncertainty given by the square root of the diagonal elements of the extracted covariance matrix. Different generator predictions are indicated by the colored lines with corresponding  $\chi^2$  values displayed in the legend. The inset provides a magnified view of the backwards bins.

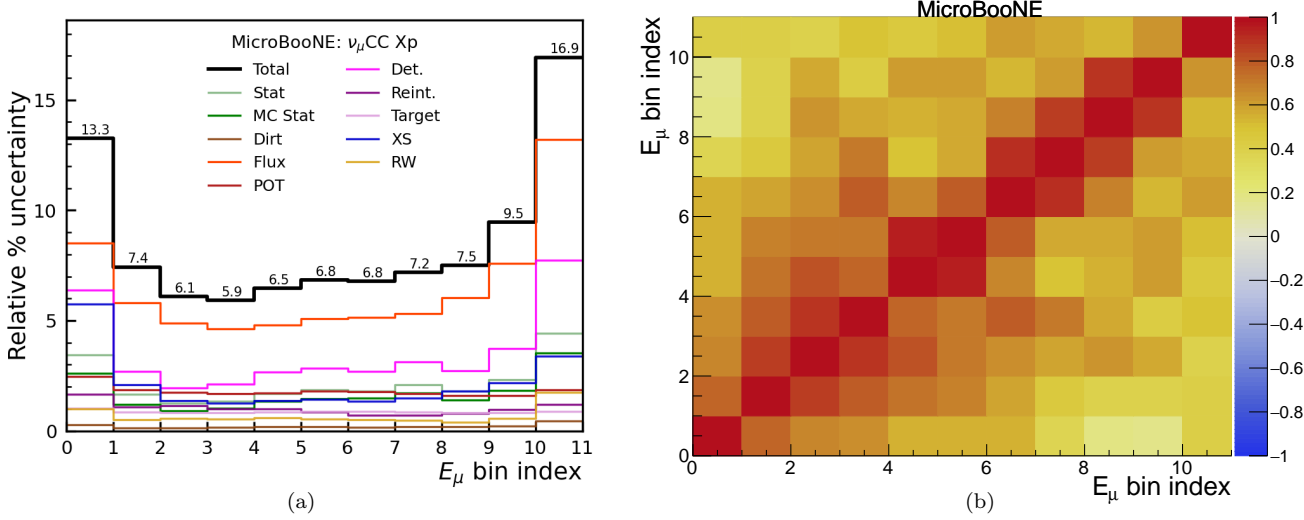

FIG. 7: (a) Contribution of uncertainties by systematic type for the extraction of the Xp differential cross section as a function of  $E_\mu$ . (b) The correlation matrix obtained from the extraction of the Xp differential cross section as a function of  $E_\mu$ . For both plots, the true bins are those found in Sec. IV and are the same as those on the extracted cross section. The entries shown in (a) correspond to the square root of the diagonal elements of the covariance matrix obtained from unfolding divided by the value of the extracted cross section for the given bin.

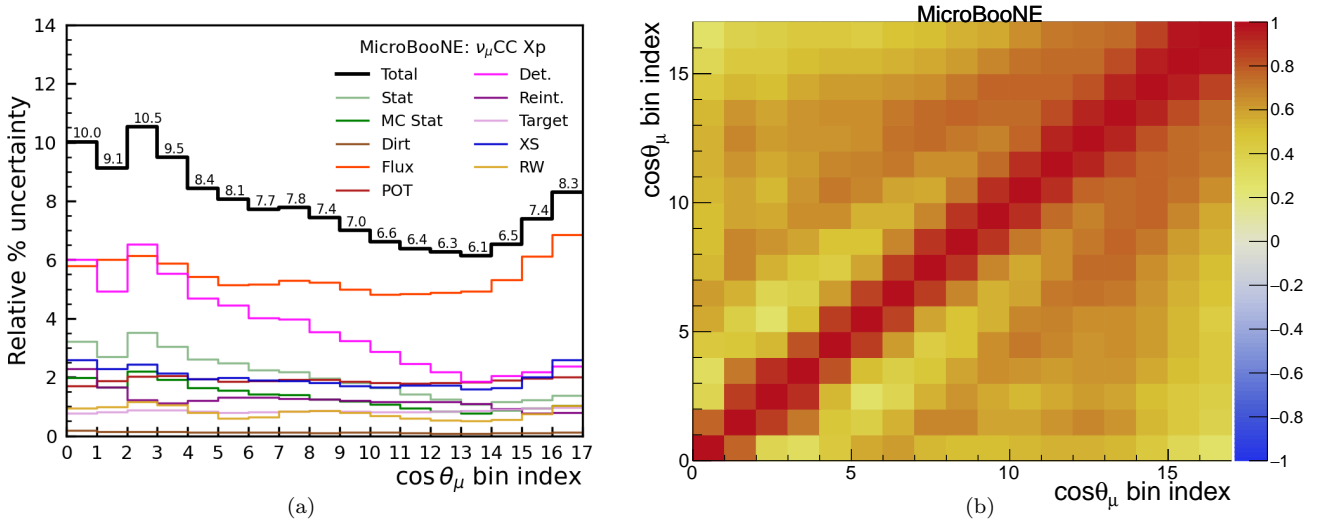

FIG. 8: (a) Contribution of uncertainties by systematic type for the extraction of the Xp differential cross section as a function of  $\cos\theta_\mu$ . (b) The correlation matrix obtained from the extraction of the Xp differential cross section as a function of  $\cos\theta_\mu$ . For both plots, the true bins are those found in Sec. IV and are the same as those on the extracted cross section. The entries shown in (a) correspond to the square root of the diagonal elements of the covariance matrix obtained from unfolding divided by the value of the extracted cross section for the given bin.

#### IV. DATA RELEASE

The unfolded cross section results shown in the main text and Sec. III can be found tabulated below. The total uncertainty, corresponding to the square root of the diagonal elements of the extracted covariance matrix, is shown for each bin. The extracted cross section results and corresponding covariance matrices can be found in a machine-readable form in `xs.txt` and `cov.txt`, respectively. The measurements from [1] are also included. The additional smearing matrix,  $A_C$ , obtained from the Wiener-SVD unfolding can be found in the same format in `Ac.txt`. Any theory or event generator prediction should be multiplied by the additional smearing matrix when comparing to this data. These files are presented in a blockwise fashion with inter-variable correlations obtained via the blockwise unfolding procedure described in [2] and in Sec. III B of [1]. The Global Bin index listed in the following tables

corresponds to the location of the bin in the blockwise covariance matrix and the Bin index corresponds to the location within the given measurement.

An example script in `gen.compare_demo.C` demonstrating how to compare the data to an external prediction is also included. This script loads the various data release files into `ROOT TMatrixD` and `TVectorD` objects. It then compares the data to an external prediction contained in `pred.txt`, which in this case is the  $\mu$ BooNE tune MC, by first smearing the prediction and then calculating  $\chi^2$  values for various measurements. More information on the files and their usage can be found in `readme.txt`.

The nominal muon neutrino flux spectrum of the Fermilab Booster Neutrino Beam at the MicroBooNE detector location can be found in `numu.flux.txt`. The results in `xs.txt` are averaged over this reference flux. External cross section predictions should likewise be averaged over this flux distribution. Note that for the total cross section reported in Fig. 25 of [1], the results are averaged over the flux from 0.2 to 4 GeV. This yields a total integrated flux of  $4.268 \times 10^{11}$  in units of number of neutrinos per  $\text{cm}^2$  for an exposure of  $6.369 \times 10^{20}$  protons on target. Similarly, for the results shown in Fig. 20 of [1], each bin is averaged over the range of the flux corresponding to the given bin. All other results have the flux integral extend over the entirety of the BNB flux. This yields a total integrated flux of  $4.586 \times 10^{11}$  in units of number of neutrinos per  $\text{cm}^2$  for an exposure of  $6.369 \times 10^{20}$  protons on target. Neutrino flux uncertainties are fully accounted for in the extracted covariance matrix and do not need to be included in theory or event generator predictions when comparing to the results. More information on `numu.flux.txt` can be found in `readme.txt`.

| $K_p$ differential cross section |     |                    |                     |                                                                                   |                                                                        |
|----------------------------------|-----|--------------------|---------------------|-----------------------------------------------------------------------------------|------------------------------------------------------------------------|
| Global Bin                       | Bin | $K_p$ Low<br>(GeV) | $K_p$ High<br>(GeV) | $\frac{d\sigma}{dK_p}$<br>( $\times 10^{-36} \frac{\text{cm}^2}{\text{Ar GeV}}$ ) | Uncertainty<br>( $\times 10^{-36} \frac{\text{cm}^2}{\text{Ar GeV}}$ ) |
| 99                               | 0   | 0                  | 0.035               | 1.9323                                                                            | 0.3621                                                                 |
| 100                              | 1   | 0.035              | 0.105               | 1.0636                                                                            | 0.1443                                                                 |
| 101                              | 2   | 0.105              | 0.1225              | 1.0174                                                                            | 0.1056                                                                 |
| 102                              | 3   | 0.1225             | 0.14                | 0.9820                                                                            | 0.0989                                                                 |
| 103                              | 4   | 0.14               | 0.1575              | 0.8981                                                                            | 0.1072                                                                 |
| 104                              | 5   | 0.1575             | 0.175               | 0.7884                                                                            | 0.0912                                                                 |
| 105                              | 6   | 0.175              | 0.1925              | 0.7312                                                                            | 0.0739                                                                 |
| 106                              | 7   | 0.1925             | 0.21                | 0.6157                                                                            | 0.0692                                                                 |
| 107                              | 8   | 0.21               | 0.245               | 0.5464                                                                            | 0.0508                                                                 |
| 108                              | 9   | 0.245              | 0.28                | 0.4212                                                                            | 0.0397                                                                 |
| 109                              | 10  | 0.28               | 0.315               | 0.3387                                                                            | 0.0322                                                                 |
| 110                              | 11  | 0.315              | 0.35                | 0.2589                                                                            | 0.0270                                                                 |
| 111                              | 12  | 0.35               | 0.42                | 0.1994                                                                            | 0.0198                                                                 |
| 112                              | 13  | 0.42               | 0.525               | 0.1136                                                                            | 0.0139                                                                 |
| 113                              | 14  | 0.525              | 0.8                 | 0.0335                                                                            | 0.0117                                                                 |

TABLE I: Unfolded  $K_p$  differential cross section result. Bin describes the binning structure for the given measurement and Global Bin describes the binning structure used in the blockwise covariance matrix. Uncertainty corresponds to the square root of the diagonal elements of the extracted covariance matrix.

| 0pNp $\cos \theta_\mu$ and $E_\mu$ double-differential cross section |     |                                |                                 |                      |                       |                                                                                                       |                                                                        |
|----------------------------------------------------------------------|-----|--------------------------------|---------------------------------|----------------------|-----------------------|-------------------------------------------------------------------------------------------------------|------------------------------------------------------------------------|
| Global Bin                                                           | Bin | $\cos \theta_\mu$ Low<br>(rad) | $\cos \theta_\mu$ High<br>(rad) | $E_\mu$ Low<br>(GeV) | $E_\mu$ High<br>(GeV) | $\frac{d^2\sigma}{d\cos\theta_\mu dE_\mu}$<br>( $\times 10^{-36} \frac{\text{cm}^2}{\text{Ar GeV}}$ ) | Uncertainty<br>( $\times 10^{-36} \frac{\text{cm}^2}{\text{Ar GeV}}$ ) |
| 0p                                                                   |     |                                |                                 |                      |                       |                                                                                                       |                                                                        |
| 138                                                                  | 0   | -1                             | -0.5                            | 0.106                | 0.226                 | 0.00652                                                                                               | 0.00227                                                                |
| 139                                                                  | 1   | -1                             | -0.5                            | 0.226                | 0.296                 | 0.01443                                                                                               | 0.00341                                                                |
| 140                                                                  | 2   | -1                             | -0.5                            | 0.296                | 2.506                 | 0.00053                                                                                               | 0.00010                                                                |
| 141                                                                  | 3   | -0.5                           | 0                               | 0.106                | 0.226                 | 0.00615                                                                                               | 0.00254                                                                |
| 142                                                                  | 4   | -0.5                           | 0                               | 0.226                | 0.296                 | 0.02031                                                                                               | 0.00415                                                                |

continued on next page

| continued from previous page |     |                       |                        |             |              |                                                       |                                                       |
|------------------------------|-----|-----------------------|------------------------|-------------|--------------|-------------------------------------------------------|-------------------------------------------------------|
| Global Bin                   | Bin | $\cos \theta_\mu$ Low | $\cos \theta_\mu$ High | $E_\mu$ Low | $E_\mu$ High | $\frac{d^2\sigma}{d\cos\theta_\mu dE_\mu}$            | Uncertainty                                           |
|                              |     | (rad)                 | (rad)                  | (GeV)       | (GeV)        | $(\times 10^{-36} \frac{\text{cm}^2}{\text{Ar GeV}})$ | $(\times 10^{-36} \frac{\text{cm}^2}{\text{Ar GeV}})$ |
| 143                          | 5   | -0.5                  | 0                      | 0.296       | 0.386        | 0.01580                                               | 0.00246                                               |
| 144                          | 6   | -0.5                  | 0                      | 0.386       | 2.506        | 0.00067                                               | 0.00010                                               |
| 145                          | 7   | 0                     | 0.3                    | 0.106       | 0.226        | 0.00554                                               | 0.00242                                               |
| 146                          | 8   | 0                     | 0.3                    | 0.226       | 0.296        | 0.02283                                               | 0.00504                                               |
| 147                          | 9   | 0                     | 0.3                    | 0.296       | 0.386        | 0.02476                                               | 0.00352                                               |
| 148                          | 10  | 0                     | 0.3                    | 0.386       | 2.506        | 0.00235                                               | 0.00043                                               |
| 149                          | 11  | 0.3                   | 0.5                    | 0.106       | 0.226        | 0.00520                                               | 0.00213                                               |
| 150                          | 12  | 0.3                   | 0.5                    | 0.226       | 0.296        | 0.02290                                               | 0.00535                                               |
| 151                          | 13  | 0.3                   | 0.5                    | 0.296       | 0.386        | 0.03408                                               | 0.00511                                               |
| 152                          | 14  | 0.3                   | 0.5                    | 0.386       | 0.505        | 0.03759                                               | 0.00634                                               |
| 153                          | 15  | 0.3                   | 0.5                    | 0.505       | 0.577        | 0.03076                                               | 0.00356                                               |
| 154                          | 16  | 0.3                   | 0.5                    | 0.577       | 2.506        | 0.00200                                               | 0.00022                                               |
| 155                          | 17  | 0.5                   | 0.7                    | 0.106       | 0.226        | 0.00533                                               | 0.00228                                               |
| 156                          | 18  | 0.5                   | 0.7                    | 0.226       | 0.296        | 0.02082                                               | 0.00618                                               |
| 157                          | 19  | 0.5                   | 0.7                    | 0.296       | 0.386        | 0.03998                                               | 0.00754                                               |
| 158                          | 20  | 0.5                   | 0.7                    | 0.386       | 0.505        | 0.06162                                               | 0.00772                                               |
| 159                          | 21  | 0.5                   | 0.7                    | 0.505       | 0.577        | 0.06453                                               | 0.00732                                               |
| 160                          | 22  | 0.5                   | 0.7                    | 0.577       | 0.659        | 0.04579                                               | 0.00535                                               |
| 161                          | 23  | 0.5                   | 0.7                    | 0.659       | 0.753        | 0.02669                                               | 0.00314                                               |
| 162                          | 24  | 0.5                   | 0.7                    | 0.753       | 0.861        | 0.01302                                               | 0.00162                                               |
| 163                          | 25  | 0.5                   | 0.7                    | 0.861       | 2.506        | 0.00094                                               | 0.00016                                               |
| 164                          | 26  | 0.7                   | 0.8                    | 0.106       | 0.296        | 0.00712                                               | 0.00289                                               |
| 165                          | 27  | 0.7                   | 0.8                    | 0.296       | 0.386        | 0.03687                                               | 0.00581                                               |
| 166                          | 28  | 0.7                   | 0.8                    | 0.386       | 0.505        | 0.07374                                               | 0.00879                                               |
| 167                          | 29  | 0.7                   | 0.8                    | 0.505       | 0.577        | 0.09042                                               | 0.00922                                               |
| 168                          | 30  | 0.7                   | 0.8                    | 0.577       | 0.659        | 0.08027                                               | 0.00927                                               |
| 169                          | 31  | 0.7                   | 0.8                    | 0.659       | 0.753        | 0.05918                                               | 0.00694                                               |
| 170                          | 32  | 0.7                   | 0.8                    | 0.753       | 0.861        | 0.03405                                               | 0.00411                                               |
| 171                          | 33  | 0.7                   | 0.8                    | 0.861       | 0.984        | 0.02128                                               | 0.00329                                               |
| 172                          | 34  | 0.7                   | 0.8                    | 0.984       | 2.506        | 0.00232                                               | 0.00042                                               |
| 173                          | 35  | 0.8                   | 0.9                    | 0.106       | 0.296        | 0.00426                                               | 0.00289                                               |
| 174                          | 36  | 0.8                   | 0.9                    | 0.296       | 0.386        | 0.02919                                               | 0.00626                                               |
| 175                          | 37  | 0.8                   | 0.9                    | 0.386       | 0.505        | 0.07524                                               | 0.01074                                               |
| 176                          | 38  | 0.8                   | 0.9                    | 0.505       | 0.577        | 0.10432                                               | 0.01162                                               |
| 177                          | 39  | 0.8                   | 0.9                    | 0.577       | 0.659        | 0.11531                                               | 0.01198                                               |
| 178                          | 40  | 0.8                   | 0.9                    | 0.659       | 0.753        | 0.10733                                               | 0.01210                                               |
| 179                          | 41  | 0.8                   | 0.9                    | 0.753       | 0.861        | 0.09633                                               | 0.00947                                               |
| 180                          | 42  | 0.8                   | 0.9                    | 0.861       | 0.984        | 0.07758                                               | 0.00803                                               |
| 181                          | 43  | 0.8                   | 0.9                    | 0.984       | 1.285        | 0.03987                                               | 0.00471                                               |
| 182                          | 44  | 0.8                   | 0.9                    | 1.285       | 2.506        | 0.00417                                               | 0.00060                                               |
| 183                          | 45  | 0.9                   | 1                      | 0.106       | 0.296        | 0.00088                                               | 0.00239                                               |
| 184                          | 46  | 0.9                   | 1                      | 0.296       | 0.386        | 0.02101                                               | 0.00740                                               |
| 185                          | 47  | 0.9                   | 1                      | 0.386       | 0.505        | 0.06760                                               | 0.01272                                               |
| 186                          | 48  | 0.9                   | 1                      | 0.505       | 0.577        | 0.09532                                               | 0.01260                                               |
| 187                          | 49  | 0.9                   | 1                      | 0.577       | 0.659        | 0.12443                                               | 0.01517                                               |
| 188                          | 50  | 0.9                   | 1                      | 0.659       | 0.753        | 0.16087                                               | 0.01426                                               |
| 189                          | 51  | 0.9                   | 1                      | 0.753       | 0.861        | 0.21292                                               | 0.01773                                               |
| 190                          | 52  | 0.9                   | 1                      | 0.861       | 0.984        | 0.22278                                               | 0.01964                                               |
| 191                          | 53  | 0.9                   | 1                      | 0.984       | 1.285        | 0.18994                                               | 0.01699                                               |

continued on next page



| continued from previous page |     |                       |                        |             |              |                                                       |                                                       |
|------------------------------|-----|-----------------------|------------------------|-------------|--------------|-------------------------------------------------------|-------------------------------------------------------|
| Global Bin                   | Bin | $\cos \theta_\mu$ Low | $\cos \theta_\mu$ High | $E_\mu$ Low | $E_\mu$ High | $\frac{d^2\sigma}{d\cos\theta_\mu dE_\mu}$            | Uncertainty                                           |
|                              |     | (rad)                 | (rad)                  | (GeV)       | (GeV)        | $(\times 10^{-36} \frac{\text{cm}^2}{\text{Ar GeV}})$ | $(\times 10^{-36} \frac{\text{cm}^2}{\text{Ar GeV}})$ |
| 240                          | 102 | 0.8                   | 0.9                    | 0.106       | 0.226        | 0.00678                                               | 0.00879                                               |
| 241                          | 103 | 0.8                   | 0.9                    | 0.226       | 0.296        | 0.06822                                               | 0.01689                                               |
| 242                          | 104 | 0.8                   | 0.9                    | 0.296       | 0.386        | 0.18117                                               | 0.02210                                               |
| 243                          | 105 | 0.8                   | 0.9                    | 0.386       | 0.505        | 0.29558                                               | 0.03151                                               |
| 244                          | 106 | 0.8                   | 0.9                    | 0.505       | 0.577        | 0.40656                                               | 0.03920                                               |
| 245                          | 107 | 0.8                   | 0.9                    | 0.577       | 0.659        | 0.45926                                               | 0.04662                                               |
| 246                          | 108 | 0.8                   | 0.9                    | 0.659       | 0.753        | 0.55078                                               | 0.05271                                               |
| 247                          | 109 | 0.8                   | 0.9                    | 0.753       | 0.861        | 0.61614                                               | 0.05275                                               |
| 248                          | 110 | 0.8                   | 0.9                    | 0.861       | 0.984        | 0.48886                                               | 0.04749                                               |
| 249                          | 111 | 0.8                   | 0.9                    | 0.984       | 1.285        | 0.29180                                               | 0.03358                                               |
| 250                          | 112 | 0.8                   | 0.9                    | 1.285       | 2.506        | 0.02866                                               | 0.00499                                               |
| 251                          | 113 | 0.9                   | 1                      | 0.106       | 0.226        | 0.00120                                               | 0.00901                                               |
| 252                          | 114 | 0.9                   | 1                      | 0.226       | 0.296        | 0.03343                                               | 0.01405                                               |
| 253                          | 115 | 0.9                   | 1                      | 0.296       | 0.386        | 0.08148                                               | 0.01665                                               |
| 254                          | 116 | 0.9                   | 1                      | 0.386       | 0.505        | 0.16937                                               | 0.01846                                               |
| 255                          | 117 | 0.9                   | 1                      | 0.505       | 0.577        | 0.20494                                               | 0.03159                                               |
| 256                          | 118 | 0.9                   | 1                      | 0.577       | 0.659        | 0.23187                                               | 0.04205                                               |
| 257                          | 119 | 0.9                   | 1                      | 0.659       | 0.753        | 0.35676                                               | 0.04281                                               |
| 258                          | 120 | 0.9                   | 1                      | 0.753       | 0.861        | 0.56180                                               | 0.04363                                               |
| 259                          | 121 | 0.9                   | 1                      | 0.861       | 0.984        | 0.45531                                               | 0.06002                                               |
| 260                          | 122 | 0.9                   | 1                      | 0.984       | 1.285        | 0.43240                                               | 0.05498                                               |
| 261                          | 123 | 0.9                   | 1                      | 1.285       | 2.506        | 0.09820                                               | 0.01936                                               |

TABLE II: Unfolded 0pNp  $\cos \theta_\mu$  and  $E_\mu$  double-differential cross section results. Bin describes the binning structure for the given measurement and Global Bin describes the binning structure used in the blockwise covariance matrix. Uncertainty corresponds to the square root of the diagonal elements of the extracted covariance matrix.

| Xp $\cos \theta_\mu$ and $E_\mu$ double-differential cross section |     |                       |                        |             |              |                                                       |                                                       |
|--------------------------------------------------------------------|-----|-----------------------|------------------------|-------------|--------------|-------------------------------------------------------|-------------------------------------------------------|
| Global Bin                                                         | Bin | $\cos \theta_\mu$ Low | $\cos \theta_\mu$ High | $E_\mu$ Low | $E_\mu$ High | $\frac{d^2\sigma}{d\cos\theta_\mu dE_\mu}$            | Uncertainty                                           |
|                                                                    |     | (rad)                 | (rad)                  | (GeV)       | (GeV)        | $(\times 10^{-36} \frac{\text{cm}^2}{\text{Ar GeV}})$ | $(\times 10^{-36} \frac{\text{cm}^2}{\text{Ar GeV}})$ |
| 386                                                                | 0   | -1                    | -0.5                   | 0.106       | 0.226        | 0.1229                                                | 0.0226                                                |
| 387                                                                | 1   | -1                    | -0.5                   | 0.226       | 0.296        | 0.1938                                                | 0.0203                                                |
| 388                                                                | 2   | -1                    | -0.5                   | 0.296       | 0.386        | 0.1358                                                | 0.0145                                                |
| 389                                                                | 3   | -1                    | -0.5                   | 0.386       | 2.506        | 0.0012                                                | 0.0004                                                |
| 390                                                                | 4   | -0.5                  | 0                      | 0.106       | 0.226        | 0.1225                                                | 0.0148                                                |
| 391                                                                | 5   | -0.5                  | 0                      | 0.226       | 0.296        | 0.2292                                                | 0.0163                                                |
| 392                                                                | 6   | -0.5                  | 0                      | 0.296       | 0.386        | 0.2393                                                | 0.0180                                                |
| 393                                                                | 7   | -0.5                  | 0                      | 0.386       | 0.505        | 0.1074                                                | 0.0125                                                |
| 394                                                                | 8   | -0.5                  | 0                      | 0.505       | 0.577        | 0.0240                                                | 0.0050                                                |
| 395                                                                | 9   | -0.5                  | 0                      | 0.577       | 2.506        | 0.0006                                                | 0.0006                                                |
| 396                                                                | 10  | 0                     | 0.3                    | 0.106       | 0.226        | 0.0911                                                | 0.0252                                                |
| 397                                                                | 11  | 0                     | 0.3                    | 0.226       | 0.296        | 0.2456                                                | 0.0271                                                |
| 398                                                                | 12  | 0                     | 0.3                    | 0.296       | 0.386        | 0.2995                                                | 0.0266                                                |
| 399                                                                | 13  | 0                     | 0.3                    | 0.386       | 0.505        | 0.3057                                                | 0.0226                                                |
| 400                                                                | 14  | 0                     | 0.3                    | 0.505       | 0.577        | 0.1576                                                | 0.0264                                                |
| 401                                                                | 15  | 0                     | 0.3                    | 0.577       | 0.659        | 0.0513                                                | 0.0084                                                |
| 402                                                                | 16  | 0                     | 0.3                    | 0.659       | 2.506        | 0.0012                                                | 0.0016                                                |
| 403                                                                | 17  | 0.3                   | 0.5                    | 0.106       | 0.226        | 0.0758                                                | 0.0318                                                |
| 404                                                                | 18  | 0.3                   | 0.5                    | 0.226       | 0.296        | 0.2386                                                | 0.0342                                                |
| 405                                                                | 19  | 0.3                   | 0.5                    | 0.296       | 0.386        | 0.3242                                                | 0.0327                                                |
| 406                                                                | 20  | 0.3                   | 0.5                    | 0.386       | 0.505        | 0.4264                                                | 0.0326                                                |
| 407                                                                | 21  | 0.3                   | 0.5                    | 0.505       | 0.577        | 0.3572                                                | 0.0317                                                |
| 408                                                                | 22  | 0.3                   | 0.5                    | 0.577       | 0.659        | 0.2707                                                | 0.0195                                                |
| 409                                                                | 23  | 0.3                   | 0.5                    | 0.659       | 0.753        | 0.1428                                                | 0.0120                                                |
| 410                                                                | 24  | 0.3                   | 0.5                    | 0.753       | 0.861        | 0.0528                                                | 0.0072                                                |
| 411                                                                | 25  | 0.3                   | 0.5                    | 0.861       | 2.506        | 0.0026                                                | 0.0014                                                |
| 412                                                                | 26  | 0.5                   | 0.7                    | 0.106       | 0.226        | 0.0619                                                | 0.0258                                                |
| 413                                                                | 27  | 0.5                   | 0.7                    | 0.226       | 0.296        | 0.2152                                                | 0.0274                                                |
| 414                                                                | 28  | 0.5                   | 0.7                    | 0.296       | 0.386        | 0.3253                                                | 0.0293                                                |
| 415                                                                | 29  | 0.5                   | 0.7                    | 0.386       | 0.505        | 0.4917                                                | 0.0362                                                |
| 416                                                                | 30  | 0.5                   | 0.7                    | 0.505       | 0.577        | 0.5129                                                | 0.0451                                                |
| 417                                                                | 31  | 0.5                   | 0.7                    | 0.577       | 0.659        | 0.5024                                                | 0.0360                                                |
| 418                                                                | 32  | 0.5                   | 0.7                    | 0.659       | 0.753        | 0.3813                                                | 0.0355                                                |
| 419                                                                | 33  | 0.5                   | 0.7                    | 0.753       | 0.861        | 0.1954                                                | 0.0278                                                |
| 420                                                                | 34  | 0.5                   | 0.7                    | 0.861       | 0.984        | 0.0758                                                | 0.0115                                                |
| 421                                                                | 35  | 0.5                   | 0.7                    | 0.984       | 2.506        | 0.0088                                                | 0.0041                                                |
| 422                                                                | 36  | 0.7                   | 0.8                    | 0.106       | 0.226        | 0.0155                                                | 0.0245                                                |
| 423                                                                | 37  | 0.7                   | 0.8                    | 0.226       | 0.296        | 0.1562                                                | 0.0265                                                |
| 424                                                                | 38  | 0.7                   | 0.8                    | 0.296       | 0.386        | 0.3147                                                | 0.0319                                                |
| 425                                                                | 39  | 0.7                   | 0.8                    | 0.386       | 0.505        | 0.4913                                                | 0.0365                                                |
| 426                                                                | 40  | 0.7                   | 0.8                    | 0.505       | 0.577        | 0.6139                                                | 0.0478                                                |
| 427                                                                | 41  | 0.7                   | 0.8                    | 0.577       | 0.659        | 0.6881                                                | 0.0528                                                |
| 428                                                                | 42  | 0.7                   | 0.8                    | 0.659       | 0.753        | 0.6334                                                | 0.0530                                                |
| 429                                                                | 43  | 0.7                   | 0.8                    | 0.753       | 0.861        | 0.4702                                                | 0.0476                                                |
| 430                                                                | 44  | 0.7                   | 0.8                    | 0.861       | 0.984        | 0.2958                                                | 0.0355                                                |
| 431                                                                | 45  | 0.7                   | 0.8                    | 0.984       | 1.285        | 0.1321                                                | 0.0168                                                |
| 432                                                                | 46  | 0.7                   | 0.8                    | 1.285       | 2.506        | 0.0201                                                | 0.0047                                                |
| 433                                                                | 47  | 0.8                   | 0.9                    | 0.106       | 0.226        | 0.0172                                                | 0.0185                                                |
| 434                                                                | 48  | 0.8                   | 0.9                    | 0.226       | 0.296        | 0.1443                                                | 0.0232                                                |

continued on next page

| continued from previous page |     |                       |                        |             |              |                                                       |                                                       |
|------------------------------|-----|-----------------------|------------------------|-------------|--------------|-------------------------------------------------------|-------------------------------------------------------|
| Global Bin                   | Bin | $\cos \theta_\mu$ Low | $\cos \theta_\mu$ High | $E_\mu$ Low | $E_\mu$ High | $\frac{d^2\sigma}{d\cos\theta_\mu dE_\mu}$            | Uncertainty                                           |
|                              |     | (rad)                 | (rad)                  | (GeV)       | (GeV)        | $(\times 10^{-36} \frac{\text{cm}^2}{\text{Ar GeV}})$ | $(\times 10^{-36} \frac{\text{cm}^2}{\text{Ar GeV}})$ |
| 435                          | 49  | 0.8                   | 0.9                    | 0.296       | 0.386        | 0.2494                                                | 0.0291                                                |
| 436                          | 50  | 0.8                   | 0.9                    | 0.386       | 0.505        | 0.3655                                                | 0.0400                                                |
| 437                          | 51  | 0.8                   | 0.9                    | 0.505       | 0.577        | 0.5536                                                | 0.0454                                                |
| 438                          | 52  | 0.8                   | 0.9                    | 0.577       | 0.659        | 0.6248                                                | 0.0572                                                |
| 439                          | 53  | 0.8                   | 0.9                    | 0.659       | 0.753        | 0.7094                                                | 0.0566                                                |
| 440                          | 54  | 0.8                   | 0.9                    | 0.753       | 0.861        | 0.7089                                                | 0.0577                                                |
| 441                          | 55  | 0.8                   | 0.9                    | 0.861       | 0.984        | 0.5810                                                | 0.0581                                                |
| 442                          | 56  | 0.8                   | 0.9                    | 0.984       | 1.285        | 0.3292                                                | 0.0288                                                |
| 443                          | 57  | 0.8                   | 0.9                    | 1.285       | 2.506        | 0.0614                                                | 0.0099                                                |
| 444                          | 58  | 0.9                   | 1                      | 0.106       | 0.226        | 0.0206                                                | 0.0194                                                |
| 445                          | 59  | 0.9                   | 1                      | 0.226       | 0.296        | 0.0865                                                | 0.0261                                                |
| 446                          | 60  | 0.9                   | 1                      | 0.296       | 0.386        | 0.1102                                                | 0.0272                                                |
| 447                          | 61  | 0.9                   | 1                      | 0.386       | 0.505        | 0.2818                                                | 0.0310                                                |
| 448                          | 62  | 0.9                   | 1                      | 0.505       | 0.577        | 0.4142                                                | 0.0465                                                |
| 449                          | 63  | 0.9                   | 1                      | 0.577       | 0.659        | 0.4093                                                | 0.0505                                                |
| 450                          | 64  | 0.9                   | 1                      | 0.659       | 0.753        | 0.6005                                                | 0.0560                                                |
| 451                          | 65  | 0.9                   | 1                      | 0.753       | 0.861        | 0.8366                                                | 0.0671                                                |
| 452                          | 66  | 0.9                   | 1                      | 0.861       | 0.984        | 0.8516                                                | 0.0730                                                |
| 453                          | 67  | 0.9                   | 1                      | 0.984       | 1.285        | 0.6476                                                | 0.0655                                                |
| 454                          | 68  | 0.9                   | 1                      | 1.285       | 2.506        | 0.1755                                                | 0.0209                                                |

TABLE III: Unfolded  $X_p \cos \theta_\mu$  and  $E_\mu$  double-differential cross section result. Bin describes the binning structure for the given measurement and Global Bin describes the binning structure used in the blockwise covariance matrix. Uncertainty corresponds to the square root of the diagonal elements of the extracted covariance matrix.

| Xp $E_\mu$ differential cross section |     |             |              |                                                       |                                                       |
|---------------------------------------|-----|-------------|--------------|-------------------------------------------------------|-------------------------------------------------------|
| Global Bin                            | Bin | $E_\mu$ Low | $E_\mu$ High | $\frac{d\sigma}{dE_\mu}$                              | Uncertainty                                           |
|                                       |     | (GeV)       | (GeV)        | $(\times 10^{-36} \frac{\text{cm}^2}{\text{Ar GeV}})$ | $(\times 10^{-36} \frac{\text{cm}^2}{\text{Ar GeV}})$ |
| 358                                   | 0   | 0.106       | 0.226        | 0.2080                                                | 0.0276                                                |
| 359                                   | 1   | 0.226       | 0.296        | 0.4137                                                | 0.0307                                                |
| 360                                   | 2   | 0.296       | 0.386        | 0.4994                                                | 0.0304                                                |
| 361                                   | 3   | 0.386       | 0.505        | 0.4652                                                | 0.0275                                                |
| 362                                   | 4   | 0.505       | 0.577        | 0.4068                                                | 0.0263                                                |
| 363                                   | 5   | 0.577       | 0.659        | 0.3455                                                | 0.0236                                                |
| 364                                   | 6   | 0.659       | 0.753        | 0.3051                                                | 0.0207                                                |
| 365                                   | 7   | 0.753       | 0.861        | 0.2730                                                | 0.0196                                                |
| 366                                   | 8   | 0.861       | 0.984        | 0.2215                                                | 0.0166                                                |
| 367                                   | 9   | 0.984       | 1.285        | 0.1226                                                | 0.0116                                                |
| 368                                   | 10  | 1.285       | 2.506        | 0.0228                                                | 0.0039                                                |

TABLE IV: Unfolded  $E_\mu$  differential cross section result. Bin describes the binning structure for the given measurement and Global Bin describes the binning structure used in the blockwise covariance matrix. Uncertainty corresponds to the square root of the diagonal elements of the extracted covariance matrix.

| Xp $\cos \theta_\mu$ differential cross section |     |                       |                        |                                                                                            |                                                                    |
|-------------------------------------------------|-----|-----------------------|------------------------|--------------------------------------------------------------------------------------------|--------------------------------------------------------------------|
| Global Bin                                      | Bin | $\cos \theta_\mu$ Low | $\cos \theta_\mu$ High | $\frac{d\sigma}{d \cos \theta_\mu}$<br>( $\times 10^{-36} \frac{\text{cm}^2}{\text{Ar}}$ ) | Uncertainty<br>( $\times 10^{-36} \frac{\text{cm}^2}{\text{Ar}}$ ) |
|                                                 |     | (rad)                 | (rad)                  |                                                                                            |                                                                    |
| 369                                             | 0   | -1                    | -0.6                   | 0.0423                                                                                     | 0.0042                                                             |
| 370                                             | 1   | -0.6                  | -0.5                   | 0.0469                                                                                     | 0.0043                                                             |
| 371                                             | 2   | -0.5                  | -0.4                   | 0.0490                                                                                     | 0.0052                                                             |
| 372                                             | 3   | -0.4                  | -0.3                   | 0.0557                                                                                     | 0.0053                                                             |
| 373                                             | 4   | -0.3                  | -0.2                   | 0.0667                                                                                     | 0.0056                                                             |
| 374                                             | 5   | -0.2                  | -0.1                   | 0.0771                                                                                     | 0.0062                                                             |
| 375                                             | 6   | -0.1                  | 0                      | 0.0883                                                                                     | 0.0068                                                             |
| 376                                             | 7   | 0                     | 0.1                    | 0.0984                                                                                     | 0.0077                                                             |
| 377                                             | 8   | 0.1                   | 0.2                    | 0.1109                                                                                     | 0.0082                                                             |
| 378                                             | 9   | 0.2                   | 0.3                    | 0.1306                                                                                     | 0.0091                                                             |
| 379                                             | 10  | 0.3                   | 0.4                    | 0.1591                                                                                     | 0.0105                                                             |
| 380                                             | 11  | 0.4                   | 0.5                    | 0.1975                                                                                     | 0.0126                                                             |
| 381                                             | 12  | 0.5                   | 0.6                    | 0.2402                                                                                     | 0.0151                                                             |
| 382                                             | 13  | 0.6                   | 0.7                    | 0.3005                                                                                     | 0.0184                                                             |
| 383                                             | 14  | 0.7                   | 0.8                    | 0.3918                                                                                     | 0.0256                                                             |
| 384                                             | 15  | 0.8                   | 0.9                    | 0.5392                                                                                     | 0.0398                                                             |
| 385                                             | 16  | 0.9                   | 1                      | 0.7085                                                                                     | 0.0588                                                             |

TABLE V: Unfolded  $\cos \theta_\mu$  differential cross section result. Bin describes the binning structure for the given measurement and Global Bin describes the binning structure used in the blockwise covariance matrix. Uncertainty corresponds to the square root of the diagonal elements of the extracted covariance matrix.

- 
- [1] P. Abratenko *et al.* (MicroBooNE Collaboration), Inclusive cross section measurements in final states with and without protons for charged-current  $\nu_\mu$ -ar scattering in MicroBooNE, arXiv preprint (2024), [arXiv:XXXXXXX \[hep-ex\]](#).  
[2] S. Gardiner, Mathematical methods for neutrino cross-section extraction, arXiv preprint (2024), [arXiv:2401.04065 \[hep-ex\]](#).
